# Supplementary material for: Linking Threat Tactics, Techniques, and Patterns with Defensive Weaknesses, Vulnerabilities and Affected Platform Configurations for Cyber Hunting
Source: arXiv:2010.00533 source file (2021-02-10)
Supplement: Supplementary file 1 [file appendix.tex]

\section{Appendix}

\subsection{Example Queries}
\label{sec:example-queries}

Given \texttt{Persistence} or any other \TACTICS, \bron can be used to retrieve the related \TECHNIQS, \ATTACKPATTERN{s} connected to the \TECHNIQS, the \WEAKNESS{es} connected to the \ATTACKPATTERN{s}, the \WEAKNESS{es} connected to the  \VULNERABILITIES, the \configs listed within \VULNERABILITIES, and the Vendor and Product field in the \config entry formatting. This powerful capability allows interesting queries to be posed of \bron by coding in e.g. Python.

Some examples are shown in Table~\ref{tab:sample_queries}.  We start, in the first row, by asking about the \configs related to \texttt{Persistence}. Our query script retrieves $1,352$ \configs, one of which is a vulnerability in the Oracle Argus Safety component of Oracle Health Sciences Applications.

We next select Oracle's product Argus Safety. It has a vulnerability that allows an attacker with low privilege and network access via HTTP to compromise Argus Safety. This can impact additional products and result in unauthorized update, insert or delete access to some of Oracle Argus Safety accessible data, as well as unauthorized read access to a subset of Oracle Argus Safety accessible data~\cite{cve20192432}. In the second row, we query
\bron for the means of attacking this vulnerability. \bron identifies 13 \TECHNIQS one of which is \texttt{T1553.004 Install Root Certificate}.

We then select Google Chrome and, in the third row, ask \bron about the attack patterns it is involved in and the tactics which an attack may be pursuing that target the browser. We find out that five different tactics can target the browser, one of which is \texttt{Privilege Escalation}. We also find out that the browser is the vulnerability endpoint of 147 attack patterns, e.g.  \texttt{UDP} \texttt{Scan}.  Since Chrome has many versions, we compare the same information in \bron about two versions in the 4th and 5th rows to see the difference in exposure. We choose a recent and older version. The older version (5.0.375.0) serves the objective of 4 tactics, while the more recent version~(v52.0.2743.82),  lists no tactics.  The more robust recent version also shows a reduction in attack patterns to 12 from the older's $120$.

%command is python path_search/path_search_BRON_db.py starting point id starting point type

\begin{table*}[!tb]
  \small
  \centering
\caption{Example queries illustrating some ways \bron can be used. (Note that only a subset of the threat data results are shown for each query.)}
\label{tab:sample_queries}
\begin{tabular}{p{7.5cm}|p{6.8cm}|p{2.7cm}}
\textbf{Query} & \textbf{Results (Abbreviated)} & \textbf{Number of Results}\\
\hline
\hline
\configs affected by \TACTIC of Persistence & \configs: Oracle hospitality, \dots & \configs: 1,352 \\
\hline
\TECHNIQS connected to CVE-2019-2432 (vulnerability in Oracle health sciences application) & \TECHNIQS: Install Root Certificate, \dots & \TECHNIQS: 13 \\
\hline
\multirow{2}{6cm}{\TACTICS and \ATTACKPATTERN{s} for Google Chrome (all versions)} & \TACTICS: privilege-escalation, \dots & \TACTICS: 5 \\
  & \ATTACKPATTERN{s}: UDP Scan, \dots & \ATTACKPATTERN{s}: 147 \\
\hline
\multirow{2}{6cm}{\TACTICS and \ATTACKPATTERN{s} for Google Chrome (version 5.0.375.0)} & \TACTICS: privilege-escalation, \dots & \TACTICS: 4 \\
 & \ATTACKPATTERN{s}: Buffer Overflow via Environmental Variables, \dots & \ATTACKPATTERN{s}: 120 \\
\hline
\multirow{2}{6cm}{\TACTICS and \ATTACKPATTERN{s} for Google Chrome (version 52.0.2743.82)} & \TACTICS: NONE & \TACTICS: 0 \\
& \ATTACKPATTERN{s}: Overflow Binary Resource File, \dots &  \ATTACKPATTERN{s}: 12 \\
\end{tabular}
%\end{adjustbox}
\end{table*}

\subsection{Vendors Analysis}

We use \bron to collect products of a vendor by parsing the CPE notation for \configs which includes the vendor, product, and version.

The data for Figure~\ref{fig:top-10-vendor-unique-tactic-heatmap} are extracted by finding the number of products of each vendor that are vulnerable to each \TACTIC. We find the set of \TACTICS reachable by any version of each product of a vendor via path tracing. If multiple versions of a product are affected by the same \TACTIC, that product is counted only once for that \TACTIC.
Similarly, the data for Figure~\ref{fig:product-browser-heatmap} are extracted by finding the number of versions of each vendor product that are vulnerable to each \TACTIC. We find the set of \TACTICS reachable by each version of a vendor product via path tracing.

The data for Figure~\ref{fig:top-10-vendor-cvss-violin} are extracted by finding the severity scores of products of each vendor. Products are referenced within \VULNERABILITIES which also have severity scores. Since a product may link to multiple \VULNERABILITIES with each \VULNERABILITY having its own severity score, we take the maximum severity score among the product's set of \VULNERABILITIES as that product's severity score. We plot the distribution of severity scores for products of each vendor.
Similarly, the data for Figure~\ref{fig:top-10-vendor-cvss-violin-tactics} are extracted by finding the severity scores of products of each vendor that are exposed to the \TACTICS of \texttt{Discovery} and \texttt{Defense Evasion}. We find the subset of products of each vendor that is reachable by the specific \TACTIC via path tracing. For that subset of products, we take the maximum severity scores of \VULNERABILITIES linked to each product as that product's severity score. We plot the distribution of severity scores for products of each vendor reachable by the \TACTICS of Discovery and Defense Evasion.
The data for Figure~\ref{fig:product-browser-all-cvss-violin} are extracted by using all severity scores of all \VULNERABILITIES linked to each vendor product.

% \TODO{Explain that when only the latest version is referenced is different from referencing the most recent version in the \config. I believe that in the former, we take the latest release version of a product and only include any \configs that mention it. The latter would always include a config, but just the most recent one.}

\subsubsection{Vendors and \TACTICS}\label{sec:vendor study}

\ResearchQ \textit{(Posed by e.g. CSO)} What is the difference in threat surface (profile) between different vendors?

Note that the vendor analysis can be biased by e.g. the reporting of versions and products from vendors. In addition, ratios would be great for comparison based on the number of products a vendor has.

In  Figure~\ref{fig:num_cpes} we pursue the idea of isolating vendor information within \bron.  How many times is a \company cited in an \config?  While some \companies are cited in a large number of \configs, most \companies are cited in many fewer. Even when referencing all versions of an \config, the vast majority of \companies have fewer than $1,000$.  When only one version of \configs is referenced, most \companies have fewer than 250 \configs. This difference shows that many \companies
are represented by multiple \configs of one product.

\begin{figure}[!bt]
  \centering
  \includegraphics[width=0.49\textwidth]{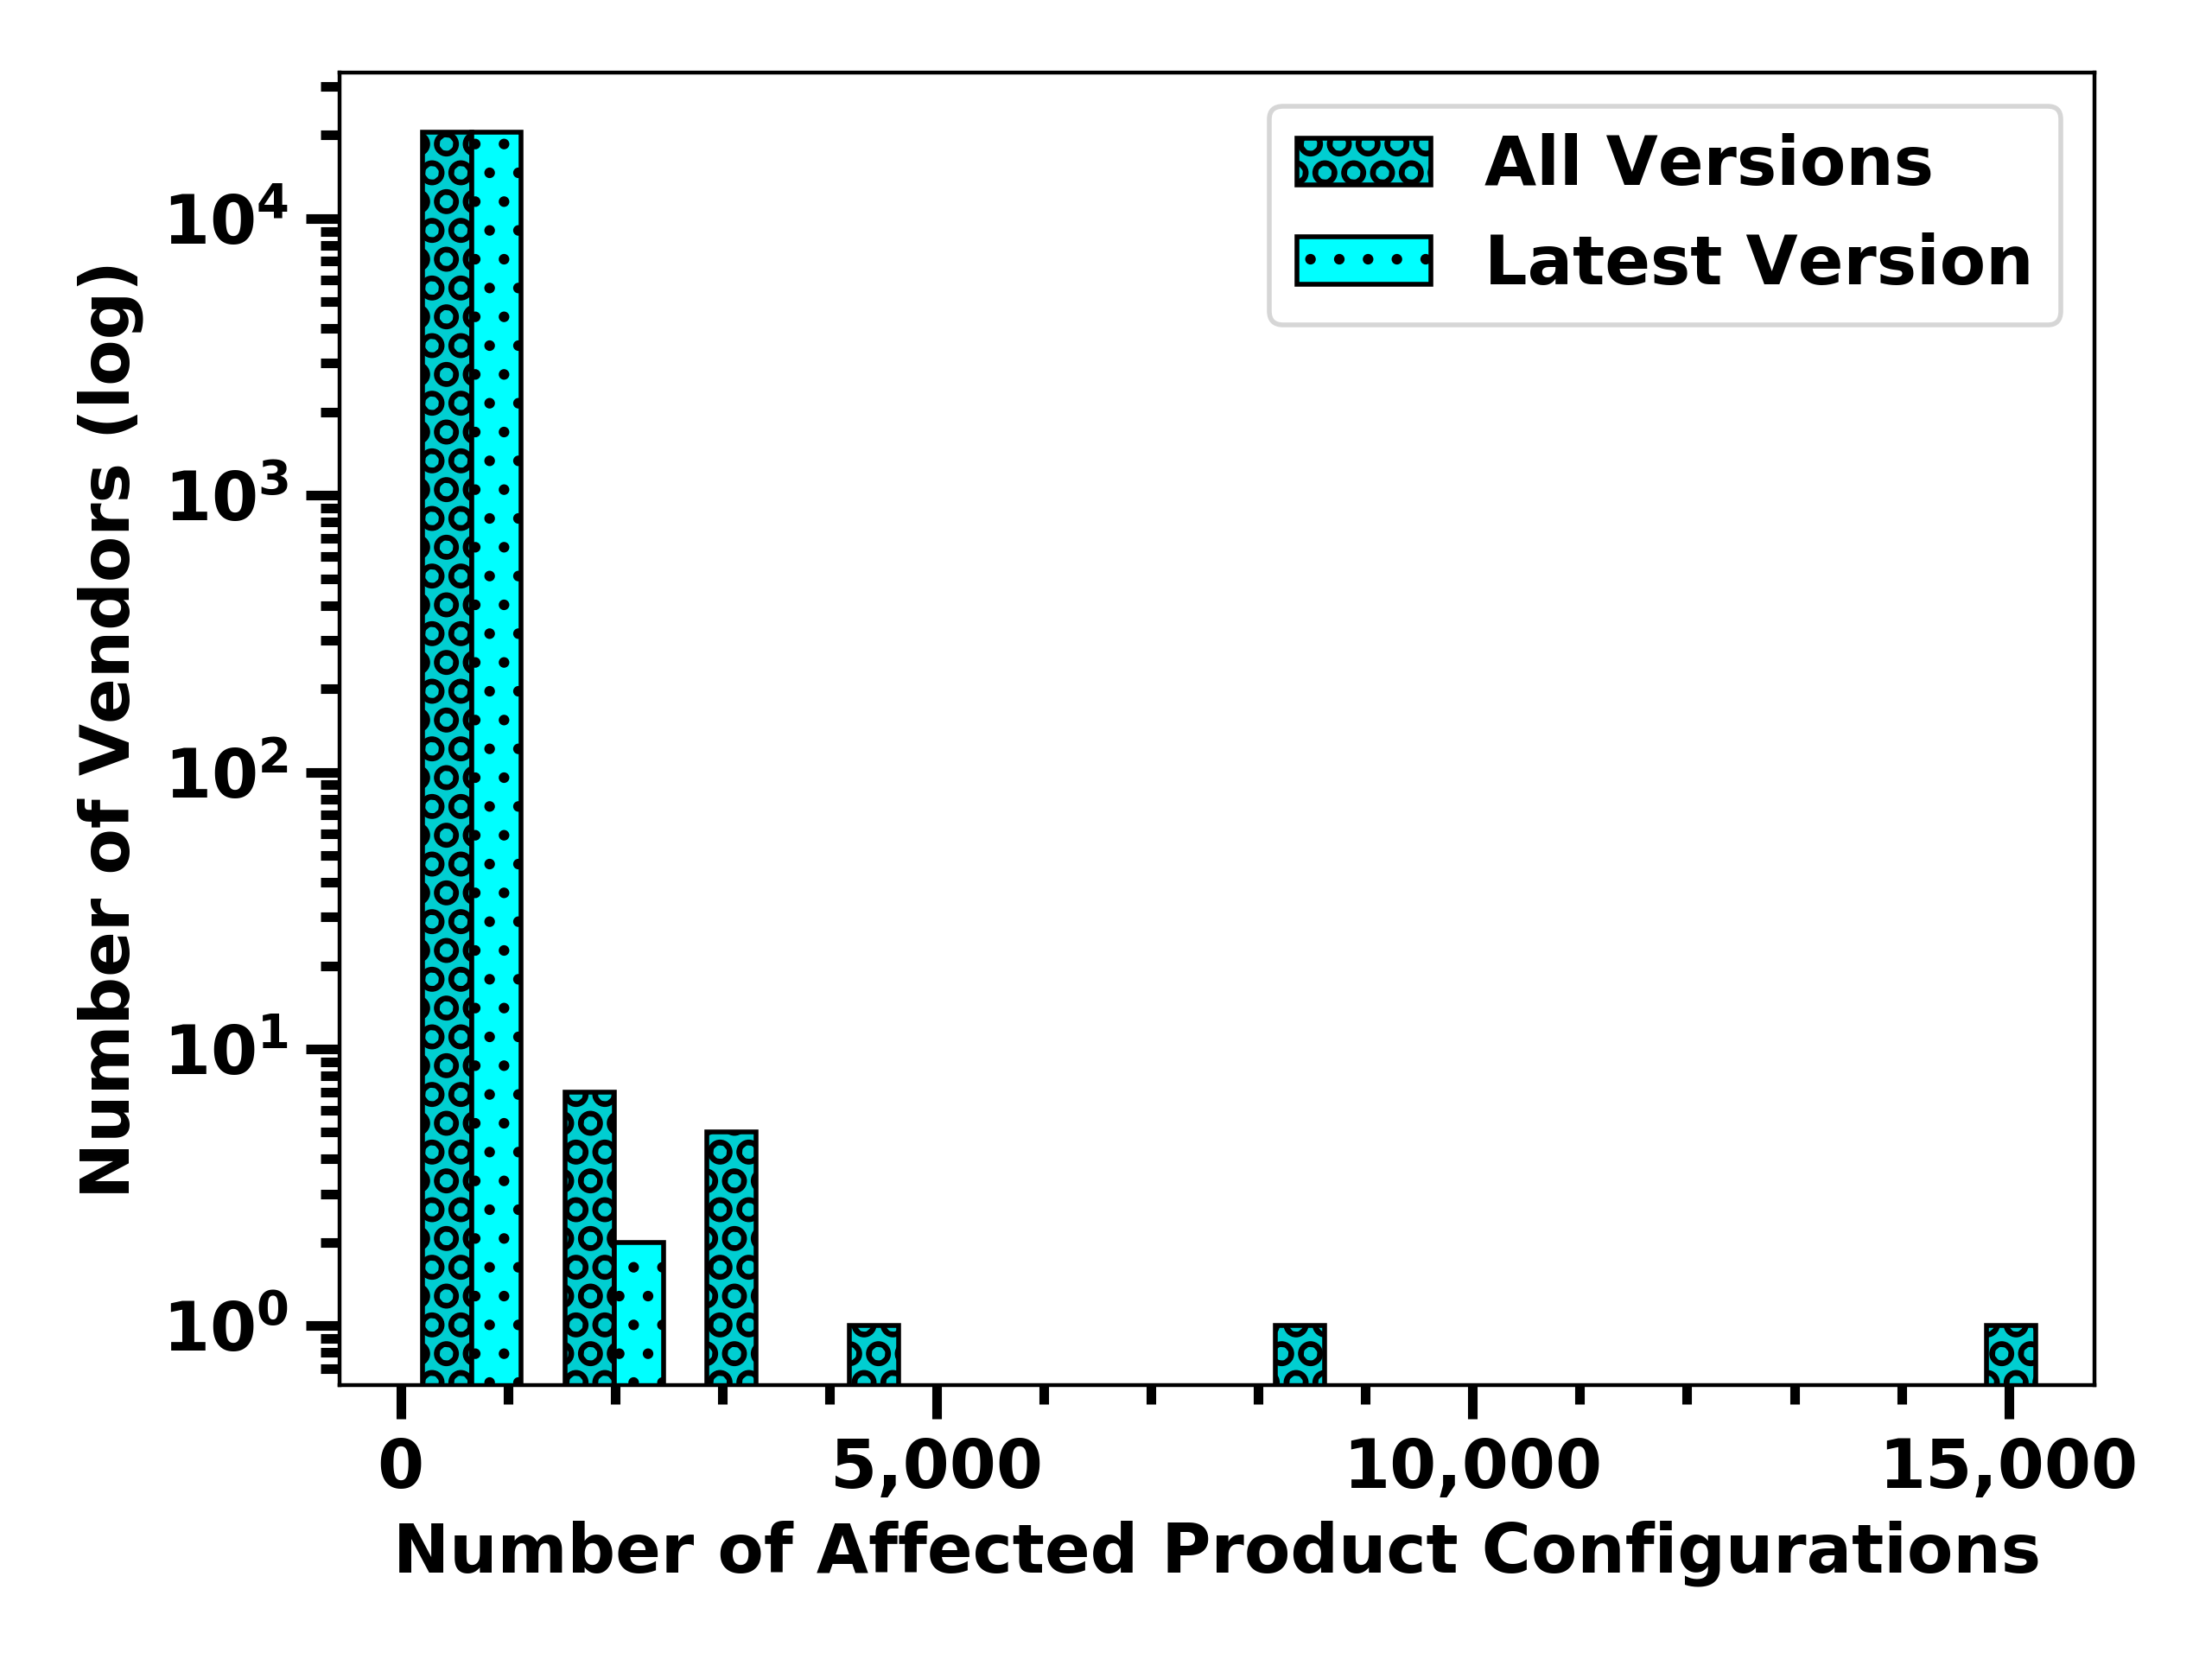}
  \caption{Number of \configs for different vendors when all versions of \configs and when only the latest version of \configs is referenced.
%X-axis is number of \configs, Y-axis is number of vendors.
}
  \label{fig:num_cpes}
\end{figure}

We decide next to focus upon a smaller set of vendors whose products have significant market share and are likely, therefore, to have significant representation in \bron.  We approximate market share by selecting the top 10 technology vendors in the Fortune 500. Members of our ``Top-10'' are Apple, Google, Microsoft, Dell, IBM, Intel, HP, Facebook, Cisco and Oracle.

Depending on \TACTIC, how many exposures do the Top-10 vendors have? Figure~\ref{fig:top-10-vendor-unique-tactic-heatmap} is a heat map that shows the number
of unique products for each vendor that are exposed to each
\TACTIC.
For each \TACTIC, looking column-wise, the map provides a count of how many different products of each vendor are vulnerable to it. A row is provided for each vendor.
Intel has many more unique products that are vulnerable to
\texttt{Defense Evasion} and \texttt{Discovery} tactical objectives compared to other \TACTICS or other vendors. For example,
Intel has $1,369$ products exposed to \texttt{Defense Evasion} and $1,084$ products
exposed to \texttt{Discovery}, while it has $54$ or fewer products  exposed to
each of the other \TACTICS. In general, more products are exposed to
\texttt{Discovery, Defense Evasion, Persistence}, and \texttt{Privilege Escalation} than
the other \TACTICS. Scanning across rows, for each vendor, we can observe how many different products are vulnerable to different \TACTICS.  Many vendors have higher vulnerability to \texttt{Persistence}, \texttt{Privilege} \texttt{Escalation} and \texttt{Defense Evasion}.  Oracle stands out with a significantly higher number of products vulnerable to \texttt{Lateral Movement}. This may be due to more documentation or to actual greater vulnerability.  The
connection analysis can help identify areas that have a lot of data,
and which have little, e.g. as in Figure~\ref{fig:top-10-vendor-unique-tactic-heatmap}.

\begin{figure}[!bt]
  \centering
  \includegraphics[width=0.49\textwidth]{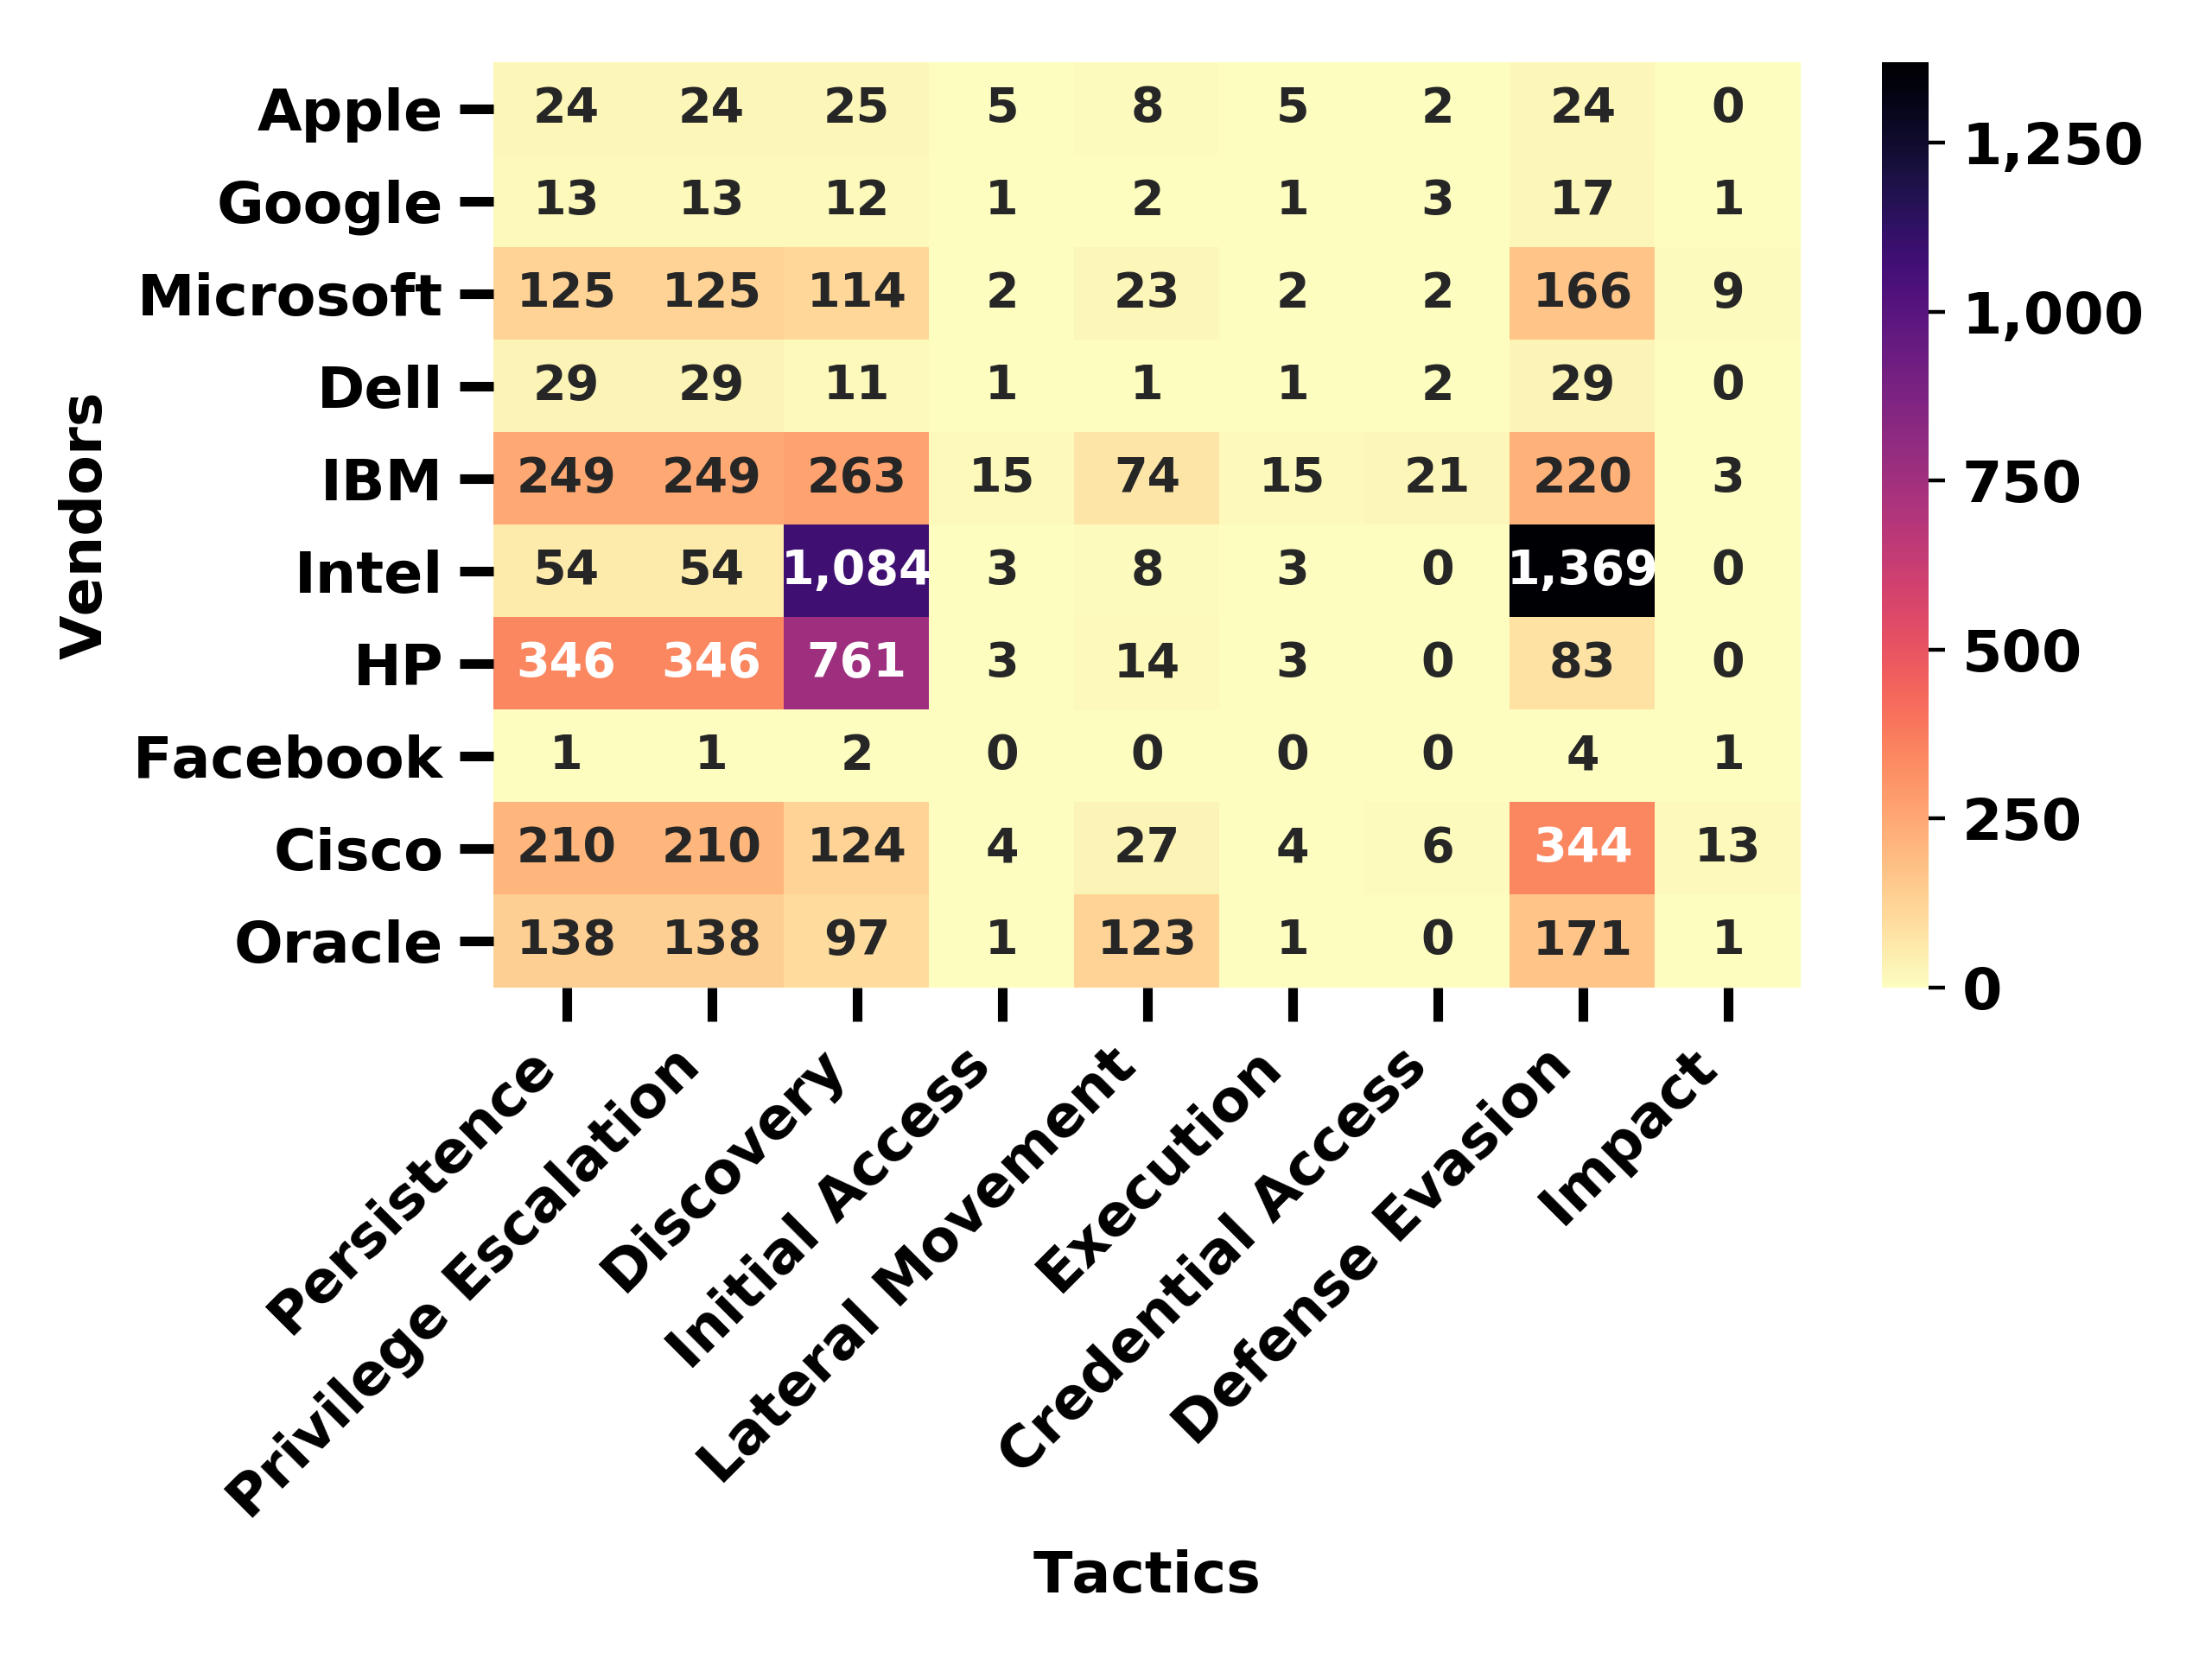}
  \caption{ Heat map showing number of unique products by vendor that are exposed to nine \TACTICS. Three \TACTICS are not shown because they did not expose any of these vendors.
%Rows are vendors, columns are \TACTICS, and value is number of unique products exposed to \TACTIC from that vendor.
Most counts are between $[0,250]$, but there are a few instances where a vendor has more than 500 unique products vulnerable to a \TACTIC.}
  \label{fig:top-10-vendor-unique-tactic-heatmap}
\end{figure}

\subsubsection{Vendors and Severity Scores}

\label{sec:vend-sever-scor}

For each vendor, we count the number of entries per source affecting them, given there are paths in \bron from \ATTACKPATTERN{s} up to \TECHNIQS.  Figure~\ref{fig:top-10-vendor-unique-bar} shows this data when all \VULNERABILITIES and all
versions of \configs are referenced. Some vendors such as Cisco and Intel
have a high \configs to \VULNERABILITY ratio, while others such as Apple have a
high \VULNERABILITY to \configs ratio.  Dell and Facebook look similar while the other vendors have similar relative \ATTACKPATTERN{s}, \VULNERABILITIES and \configs. For \TACTICS and \TECHNIQS, Facebook has fewer entries while the other nine are roughly equal.  There is also a very similar count of \ATTACKPATTERN{s} across all vendors within \bron.

\begin{figure}[!bt]
  \centering
  \includegraphics[width=0.49\textwidth]{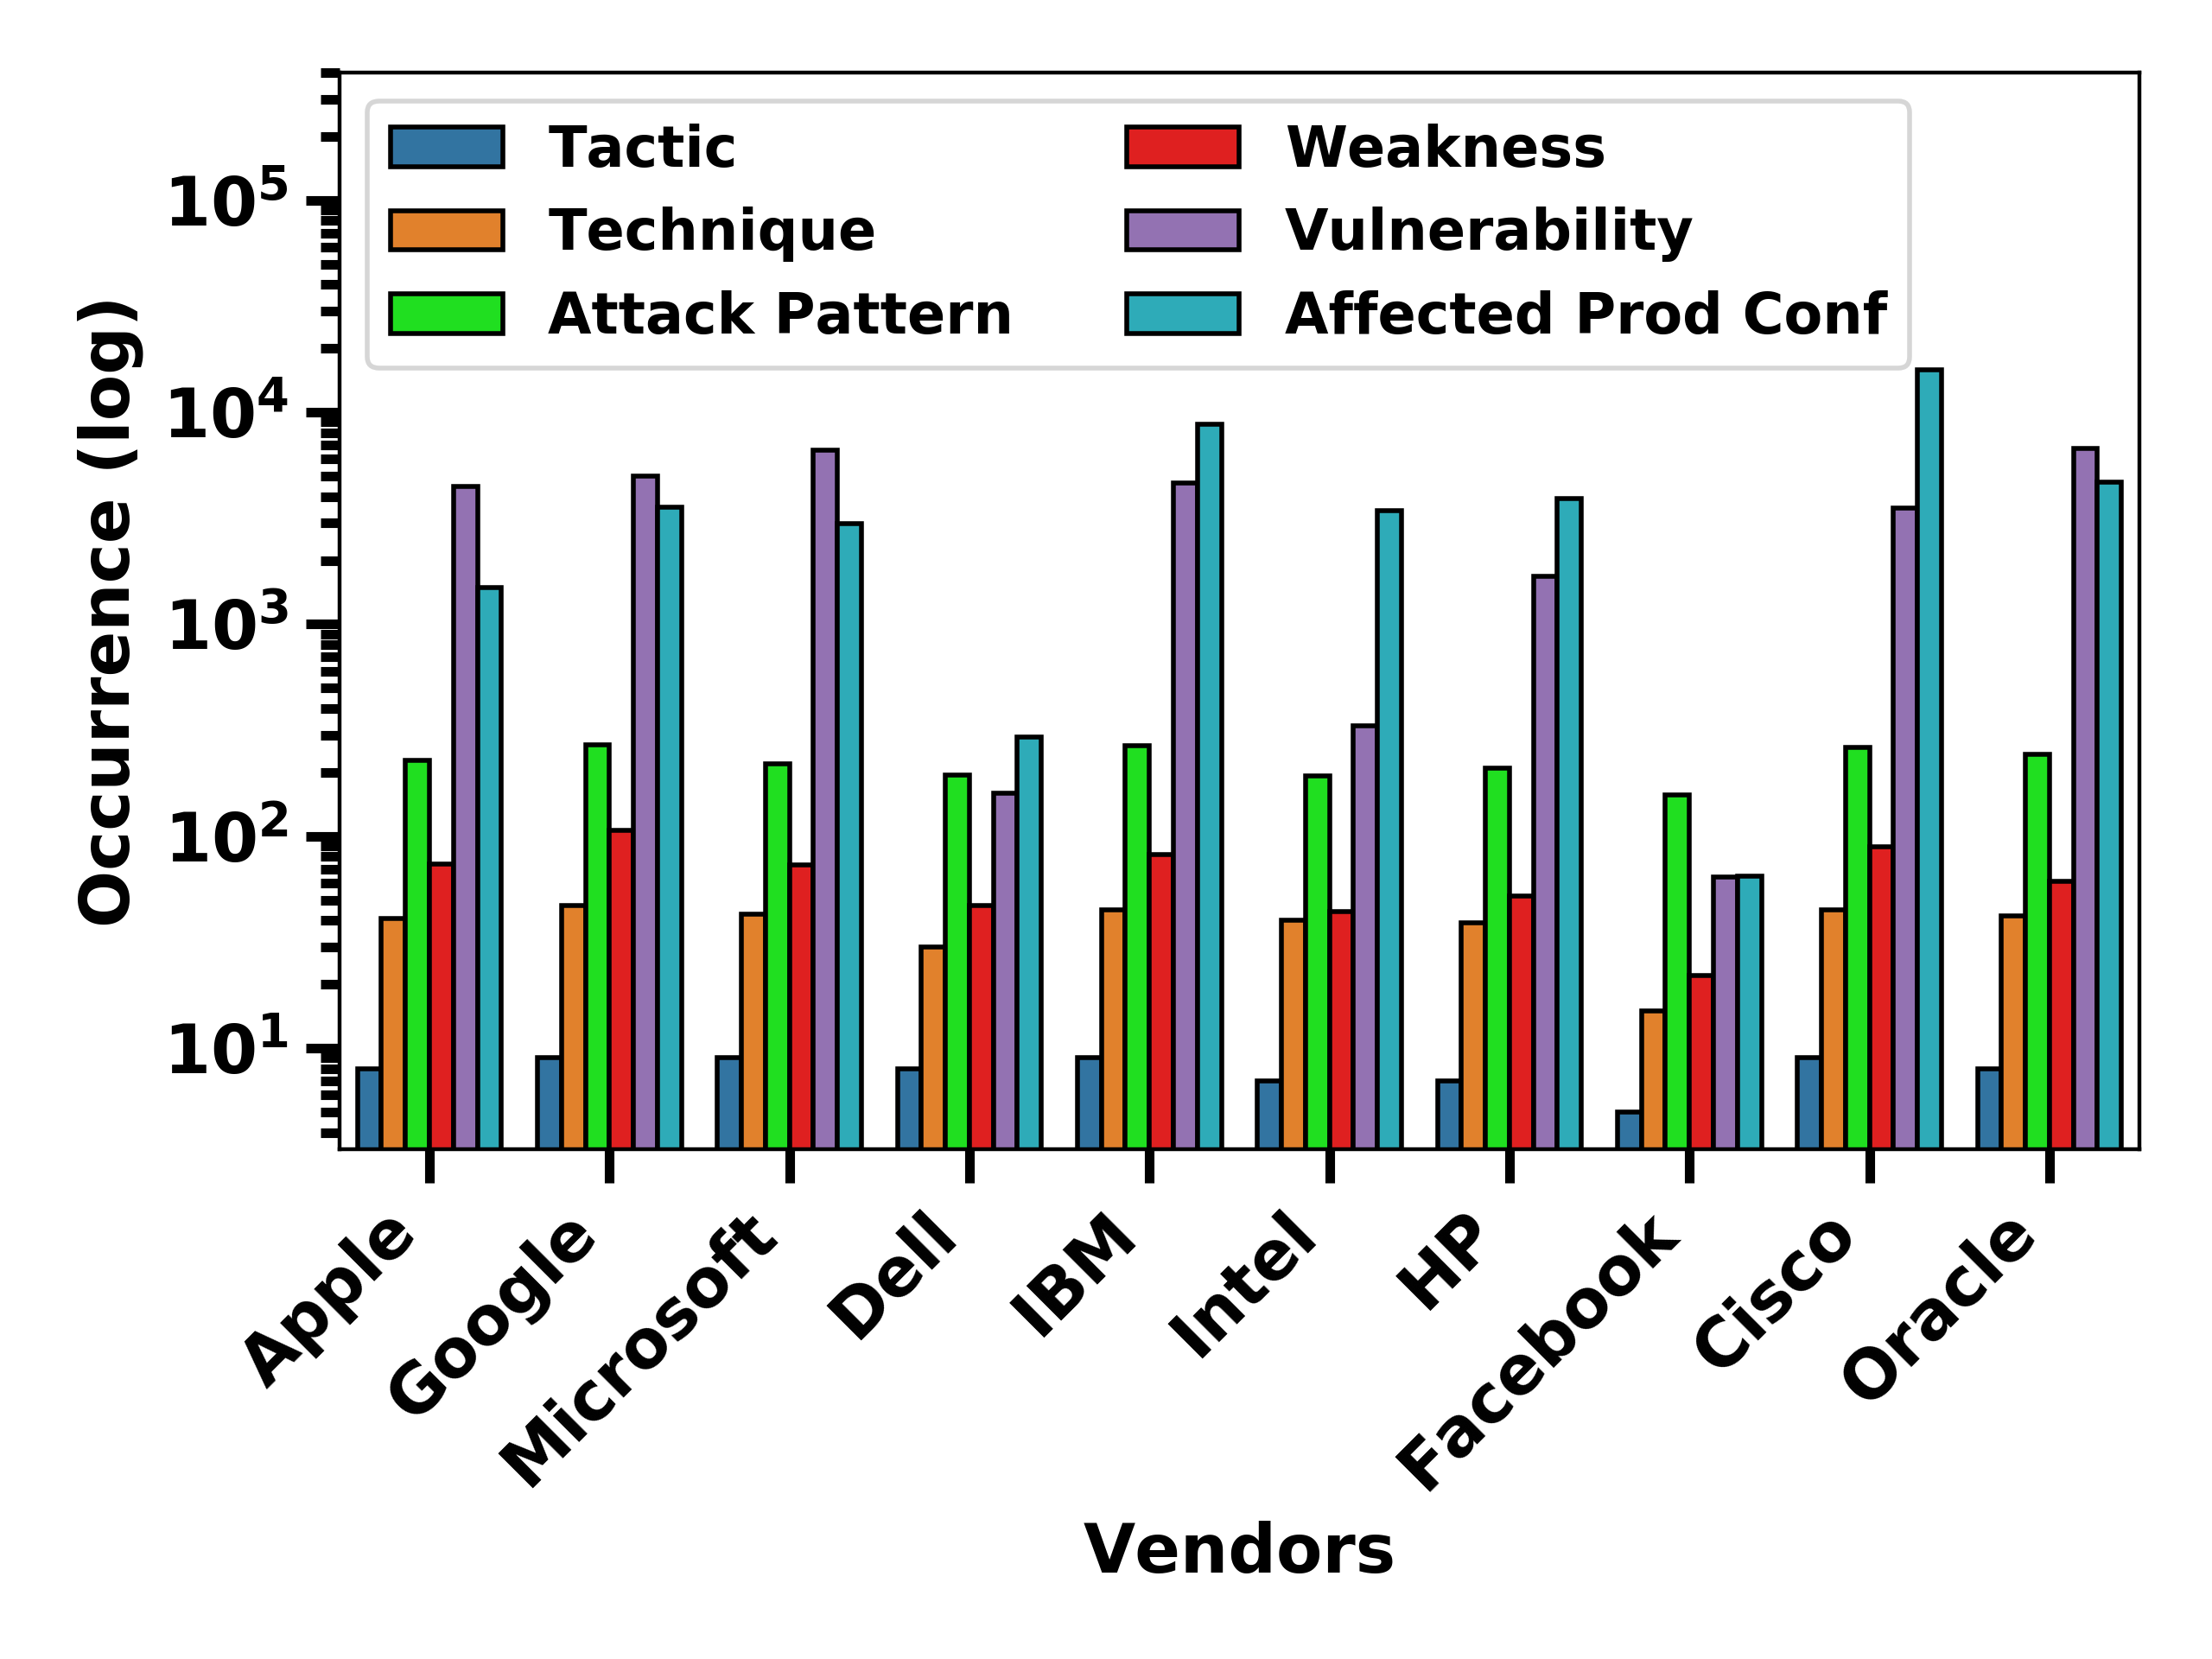}
  \caption{Number of entries per source for Top-10 \companies.
%X-axis is vendor,
%Y-axis is number of different unique entries.
%Color indicates \config, \VULNERABILITY, \WEAKNESS, \ATTACKPATTERN, \TECHNIQ, or \TACTIC.
}
  \label{fig:top-10-vendor-unique-bar}
\end{figure}

We also check the number of \configs a particular vendor incurs over time (no figure shown). It is not
distributed equally across years. \Companies, like Google
and HP, appear to have very few \configs
before 2015.
This raises a warning about making sure cross-vendor comparisons are on similar bases.  Referencing data at the same date, after the same number of versions, at the start or end of a release version would help with this.

We next consider the severity of \VULNERABILITIES of this set of vendors.   Figure~\ref{fig:top-10-vendor-cvss-violin} shows the distribution of severity scores
of vendor products across all \TACTICS, collecting the maximum \VULNERABILITY severity score of all versions. The distributions across vendors are significantly
different. Some vendors such as Google have more \configs with severity
scores around $7$ and $10$. In contrast, the distribution for Intel shows
three main peaks with severity scores between $3$ and $7$, which indicates
that Intel tends to have \configs with low and medium  severity.

We noted significantly larger counts of products exposed to the \TACTICS of \texttt{Discovery} and \texttt{Defense Evasion}. In Figure~\ref{fig:top-10-vendor-cvss-violin-tactics} we compare the corresponding distributions of severity scores.   We see that severity is distributed somewhat the same (see symmetry in the violin plot along the vertical-axis) for Apple, Google, Dell and Oracle but we see differences for the other vendors.  The question of what products specifically fall prey to these tactics and their specific severity score distributions is a topic of future work.

The severity score distribution for \configs connected to specific \TACTICS is sometimes different than severity score distribution for all \configs of a vendor. For example, the severity score distribution for Intel's \platforms connected to the \TACTIC of \texttt{Discovery} remains similar to its distribution when connected to all \platforms. However, the severity scores for Intel's \platforms connected to the \TACTIC of \texttt{Defense Evasion} is mostly near a score of 4.

\begin{figure}[tb]
  \begin{subfigure}{0.48\textwidth}
    \centering
  \includegraphics[width=\textwidth]{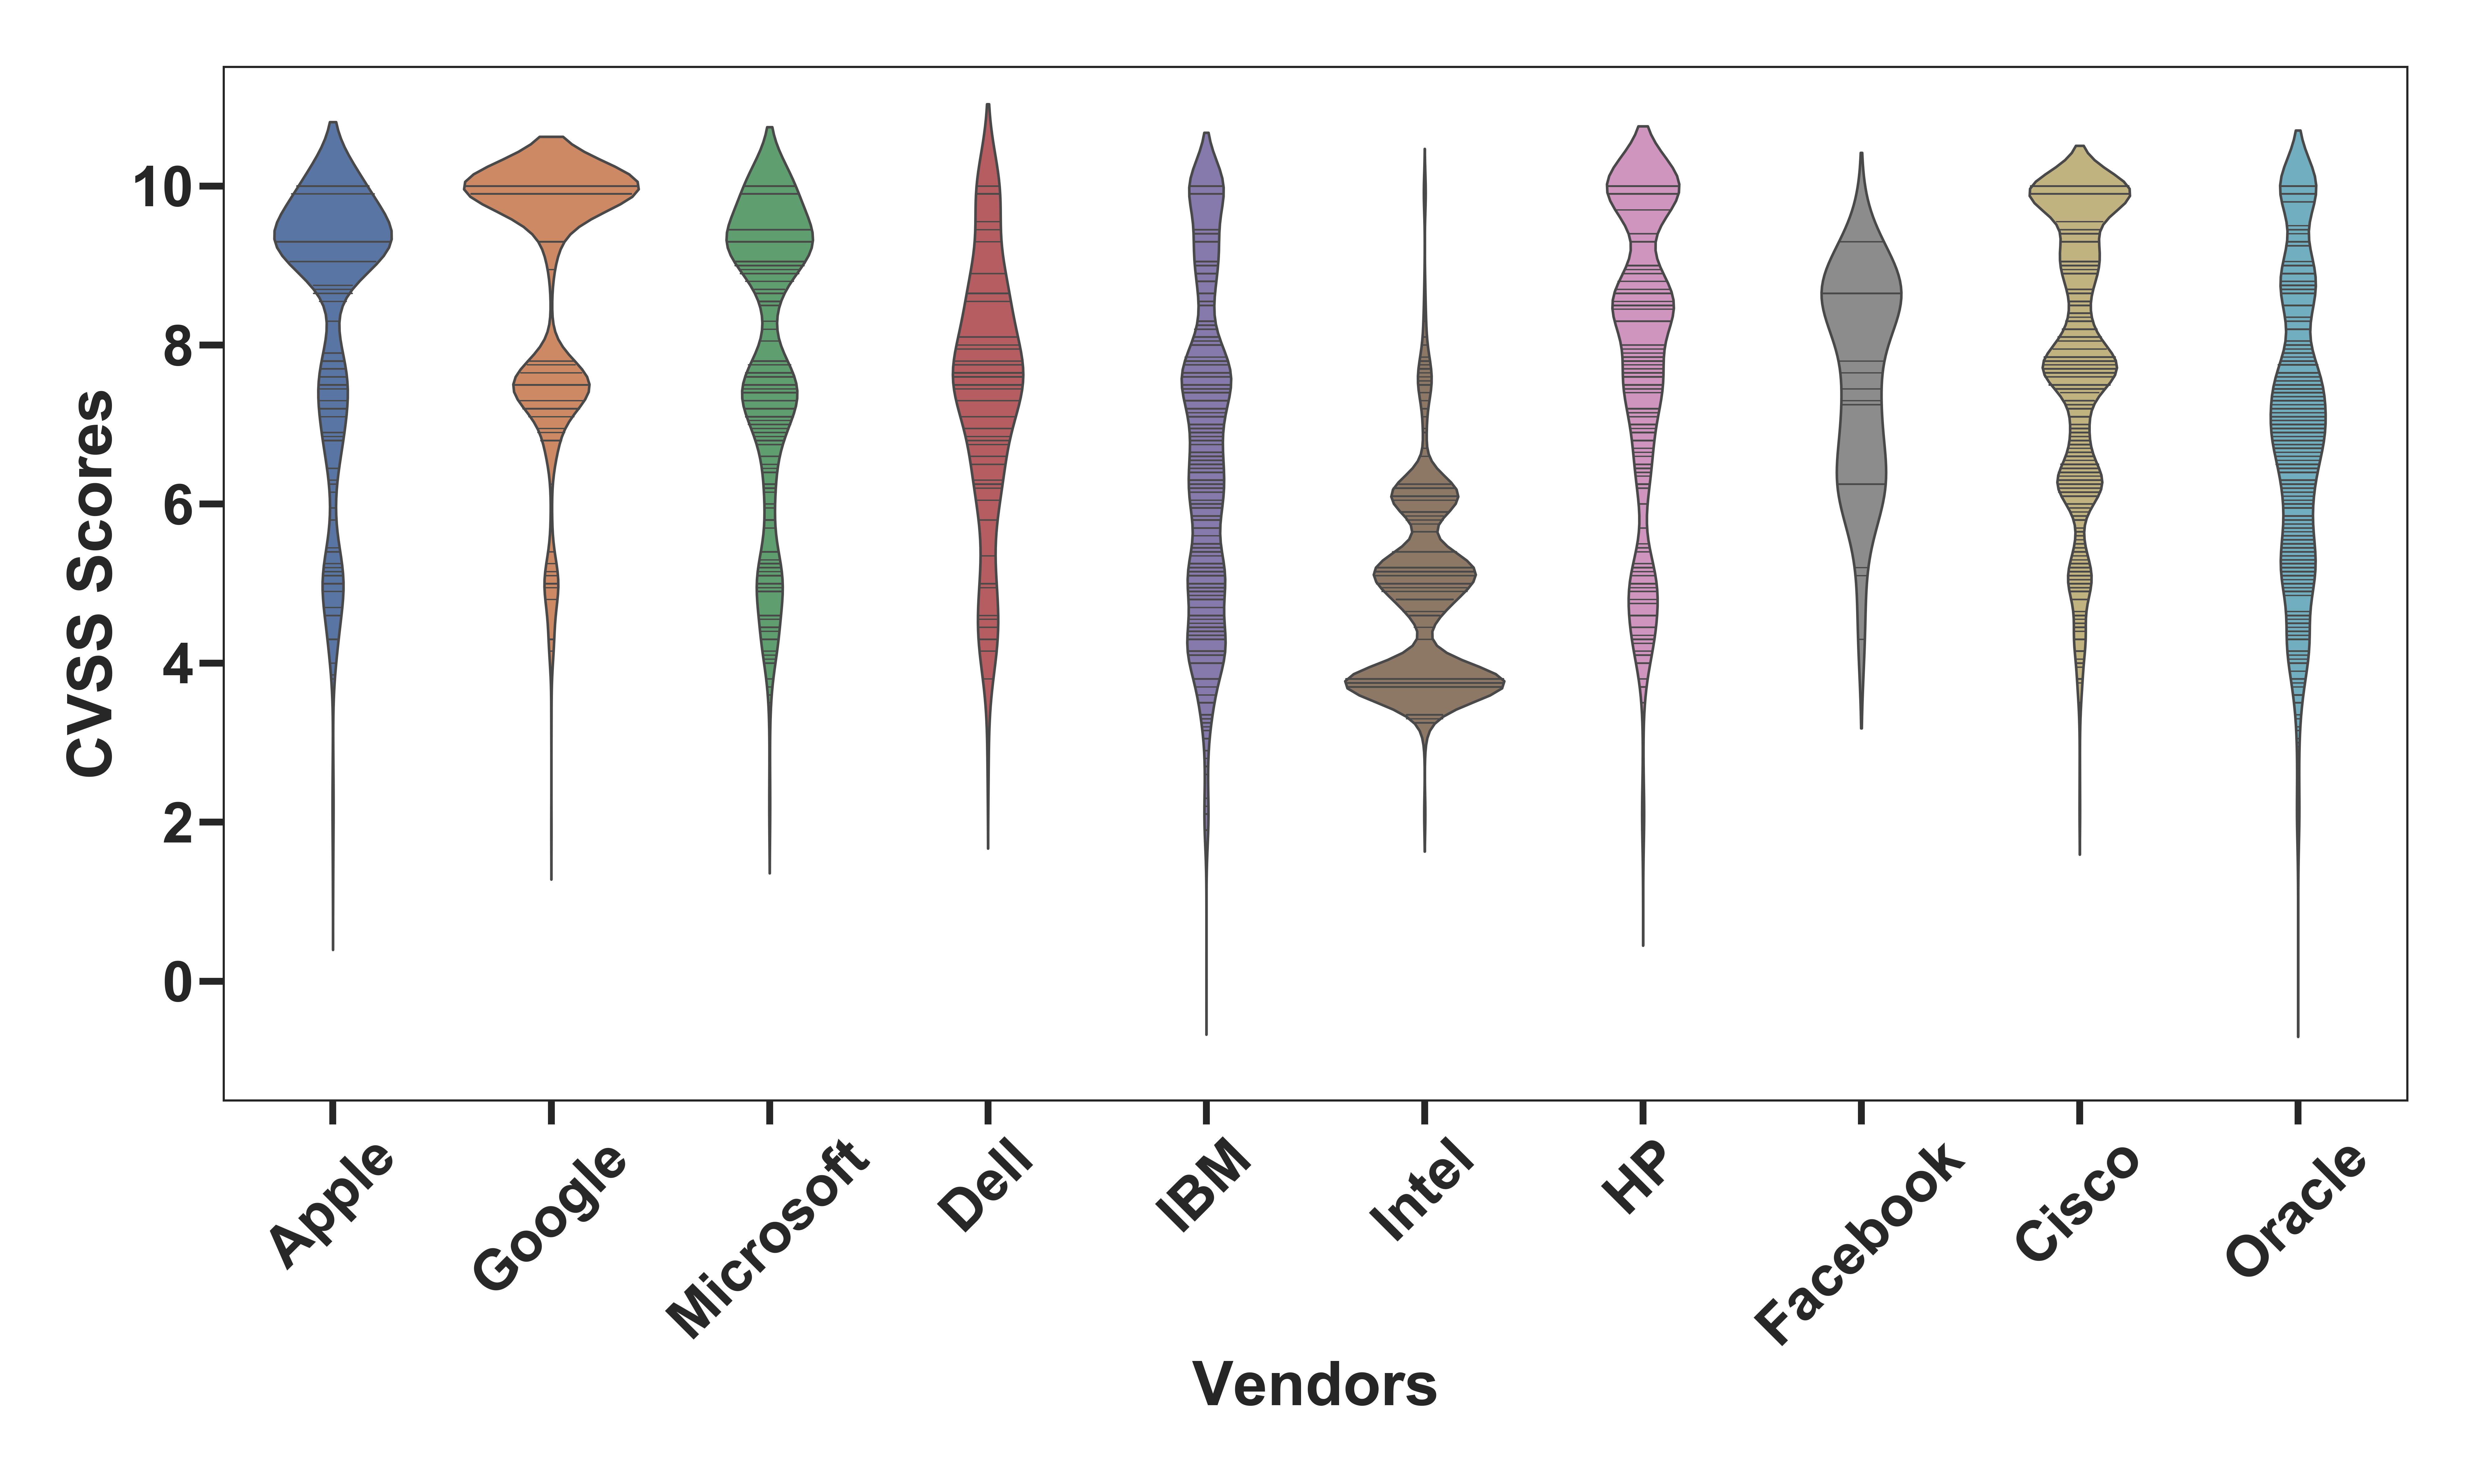}
  \caption{Distributions of severity scores for \configs connected to all \TACTICS.}
  \label{fig:top-10-vendor-cvss-violin}
\end{subfigure}

  \begin{subfigure}{0.48\textwidth}
    \centering
  \includegraphics[width=\textwidth]{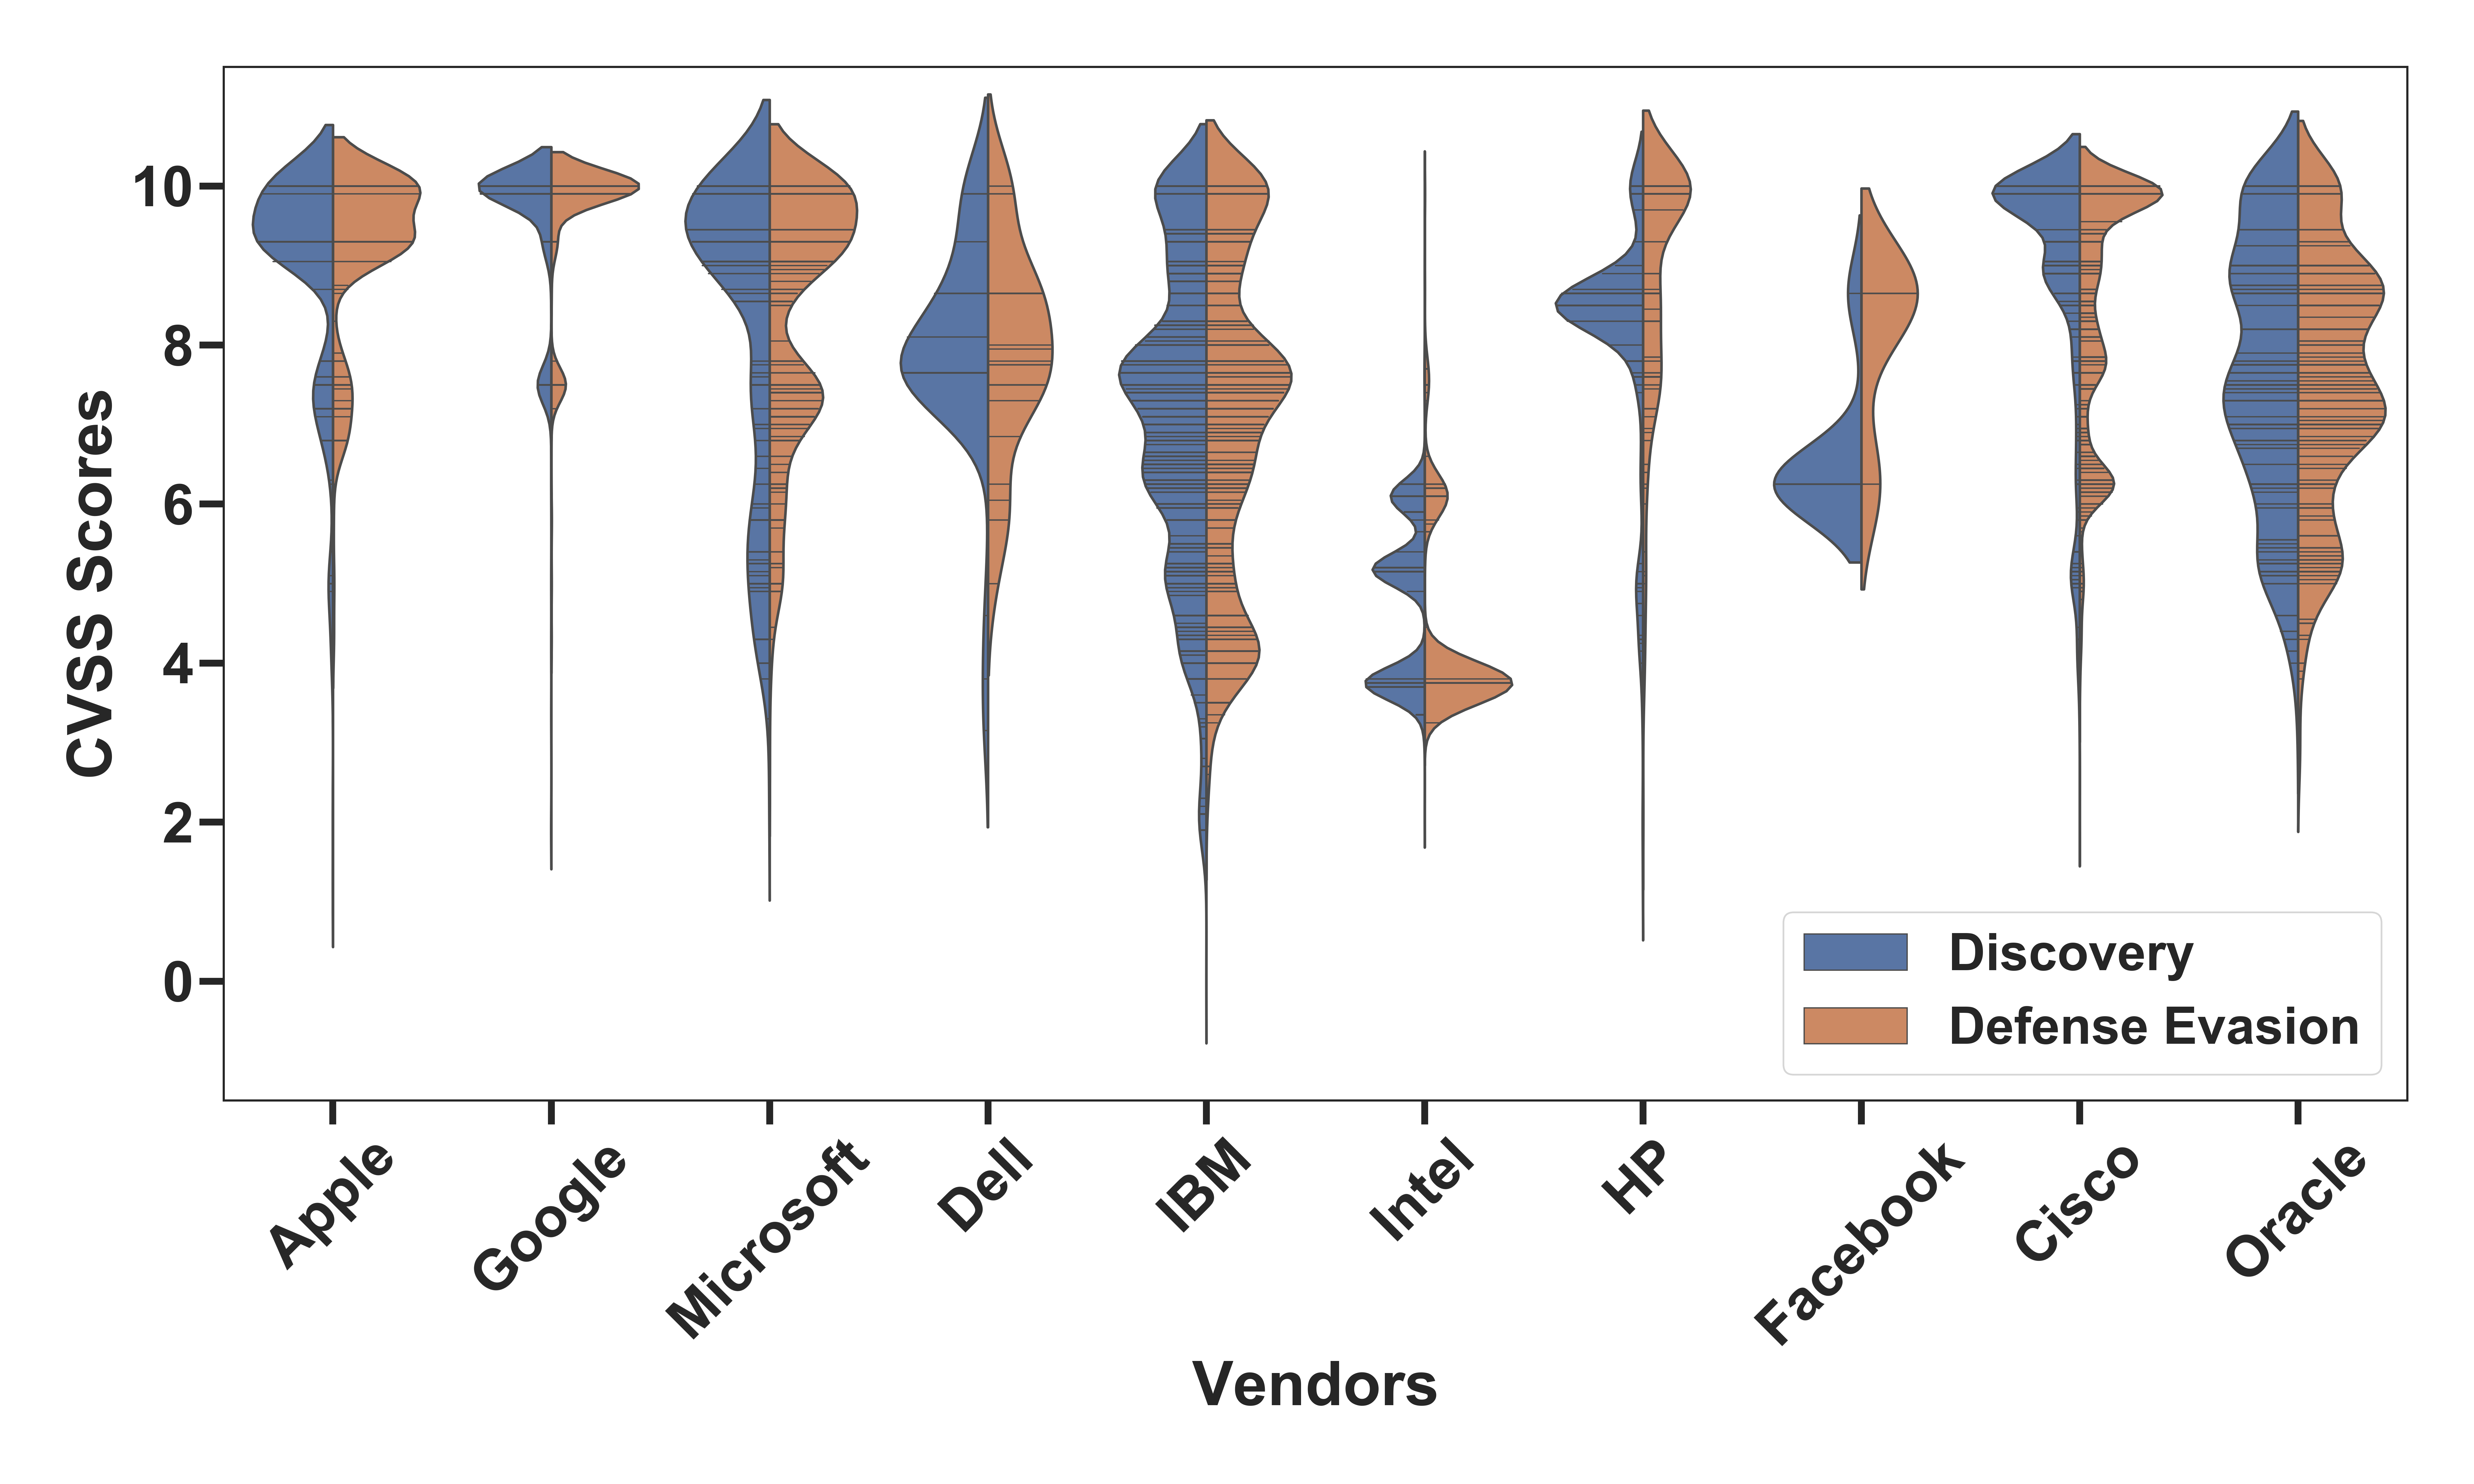}
  \caption{Distributions of severity scores for \configs connected to two specific tactics: \texttt{Discovery} (blue) and \texttt{Defense Evasion} (brown).}
  \label{fig:top-10-vendor-cvss-violin-tactics}
\end{subfigure}
\caption{Distributions of severity scores, Top-10 vendors.}
\end{figure}
